# Supplementary material for: Graphons, mergeons, and so on!
Source: arXiv:1607.01718 source file (2017-05-22)
Supplement: Supplementary file 1 [file generalclusters.tex]

\section{Clusters in general graphons}

So far we have only considered graphons defined on the unit interval with
Lebesgue measure. The notion of a graphon can be generalized:

\begin{defn}
    A \term{general graphon} is a pair $(J, W)$, where $J = (\Omega, \Sigma,
    \mu)$ is a probability space and $W : \Omega \times \Omega \to [0,1]$ is a
    symmetric, $\Sigma \times \Sigma$-measurable function.
\end{defn}

We may also generalize the procedure of sampling a graph from a general graphon.
Whereas before we sampled a graph of size $n$ by drawing $n$ points $x_1,
\ldots, x_n$ at random from the uniform distribution on $[0,1]$, we now draw $n$
points from $J$. As before, we create an empty graph with nodes labeled $1,
\ldots, n$, and connect nodes $i$ and $j$ with probability $W(x_i, x_j)$.
Therefore, any general graphon defines a random graph model. If two general
graphons define the same random graph model, we say that they are \term{weakly
isomorphic}. It is known that every general graphon on a probability space
$(\Omega, \Sigma, \mu)$ is weakly isomorphic to a graphon on the unit interval
with Lebesgue measure.

As before, we may relate graphons via measure preserving maps. Let $J$ and $J_1$
be probability spaces, and suppose $\varphi : J_1 \to J$ is measure preserving.
If $W$ is a graphon on $J$, we define its \term{pullback} $W^\varphi$ by
$W^\varphi(x,y) = W(\varphi(x), \varphi(y))$. It is clear that $W^\varphi$
is a graphon on $J$. Furthermore, a sufficient (but not necessary) condition for
$(J, W)$ and $(J_1, W_1)$ being weakly isomorphic is that $W$ is the pullback
$W_1^\varphi$ of by some measure preserving $\varphi : J \to J_1$.

As an example, consider the constant graphon $W_1 = \alpha$ defined on the unit
interval with Lebesgue measure. Suppose $W_2 = \alpha$ is defined on the finite
probability space containing a single element $q$ whose probability is
necessarily one. Clearly these two graphons define the same random graph model,
and so are weakly isomorphic. In fact, let $\varphi : [0,1] \to \{q\}$ be the
map $x \mapsto q$ for any $x \in [0,1]$. Then $\varphi$ is measure preserving,
and we have that $W_1 = W_2^\varphi$.

We may translate our definition of a graphon's clusters from the case of the
uniform distribution to a general probability space without much extra work. We
need only take into account the fact that a general probability space may
contain \term{atoms}, i.e., sets of positive measure which contain no measurable
subsets of lesser, but still positive measure.

\begin{defn}
    Let $(\Omega, \Sigma, \mu, W)$ be a general graphon. A set $C \in \Sigma$ is
    \term{disconnected at level $\lambda$} in $W$ if either
    \begin{enumerate}
        \item $C$ is an atom and $W < \lambda$ a.e. on $C \times C$, or
        \item there exists a measurable set $S \subset C$ such that $0 <
            \mu(S) < \mu(C)$ and $W < \lambda$ a.e. on $S \times (C \setminus
            S)$.
    \end{enumerate}
    Otherwise we say that $C$ is connected at level $\lambda$.
\end{defn}

The remainder of our definitions follow immediately: If $A_1$ and $A_2$ are
measurable sets with positive measure, we say that $A_1$ is connected to $A_2$
at level $\lambda$ -- written $A_1 \clusteredwith_\lambda A_2$ -- if there exists
a set $C \in \Sigma$ with $A_1 \cup A_2 \subset C$, and $C$ is connected at
level $\lambda$. It is clear that $\clusteredwith_\lambda$ is an equivalence
relation on the collection of measurable sets which are connected at level
$\lambda$, and, as before, we define the \term{clusters} at level $\lambda$ of
the general graphon to be the essential maxima of the equivalence classes.
