# Supplementary material for: Graphons, mergeons, and so on!
Source: arXiv:1607.01718 source file (2017-05-22)
Supplement: Supplementary file 6 [file twinfree.tex]

\section{Twin-free graphons}

Let $(\Omega, \Sigma, \mu, W)$ be a graphon. Two points $x, x' \in \Omega$ are
\term{twins} if $W(x,y) = W(x',y)$ for almost all $y \in \Omega$. We say that a
graphon is \term{twin-free} if no two distinct points in $\Omega$ are twins.
We say that a set $A$ separates twins $x$ and $x'$ if $|\{ x,x' \} \cap A| = 1$.

It turns out that for every graphon $(J,W)$ there exists a twin-free graphon
$(J_1, W_1)$ such that $W$ and $W_1$ are weakly isomorphic. In fact, we can
construct a measure preserving map $\psi : J \to J_1$ such that $W = W_1^\psi$
almost everywhere. The idea is to map each point in $J$ to its equivalence class
under the twin relation, so that if $x$ and $x'$ are twins, $\psi(x) =
\psi(x')$.

More formally, suppose $(\Omega, \Sigma, \mu, W)$ is a graphon. Let $\Omega_1$
be the set of equivalence classes under the twin relation on $\Omega$, and write
$\psi(x)$ denote the equivalence class containing $x$.
\[
    \Sigma_1 = \{ \psi(X) : X \in \Sigma, X \text{ does not separate twins in
    $W$} \}.
\]
Furthermore, we define the measure $\mu_1(A) = \mu(\psi^{-1}(A))$ for $A \in
\Sigma_1$. It can be shown that, with this measure, $\psi$ is measure
preserving. One may also construct a $W_1$ defined on $(\Omega_1, \Sigma_1,
\mu_1)$ such that $W_1^\psi = W$ almost everywhere.

\begin{claim}
    Suppose $A \subset \Omega$ does not separate twins. Then $\psi^{-1}(\psi(A))
    = A$ and $A$ is $\Sigma$-measurable.
\end{claim}

\begin{proof}
    It is clear that $A \subset \psi^{-1}(\psi(A))$. Now let $x \in
    \psi^{-1}(\psi(x))$. Then there exists a $y \in A$ such that $\psi(x) =
    \psi(y)$. But then $x$ and $y$ are twins. Since $A$ does not separate twins,
    $x \in A$, proving that $A = \psi^{-1}(\psi(A))$.

    Now we prove that $A$ is $\Sigma$-measurable. $\psi$ is a measurable
    function, and so the inverse image of any $\Sigma_T$-measurable set is
    $\Sigma$-measurable.  We have that $\psi(A)$ is $\Sigma_T$-measurable, since
    $A$ does not separate twins. Hence $\psi^{-1}(\psi(A)) = A$ is
    $\Sigma$-measurable.
\end{proof}

\begin{claim}
    Let $A \subset \Omega$. Then $\psi^{-1}(\psi(A))$ is $\Sigma$-measurable.
\end{claim}

\begin{proof}
    It is clear that $\psi^{-1}(\psi(A))$ does not separate twins. Hence it is
    $\Sigma$-measurable by the previous claim.
\end{proof}

\begin{defn}
    Let $(J, W)$ be a graphon, and let $J_T = (\Omega_T, \Sigma_T, \mu_T)$ be
    the corresponding twin measure space. Let $\psi : J \to J_T$ be the map
    taking $x \in J$ to its equivalence class of twins. For any $J$-measurable
    set $C$, construct the collection
    \[
        \mathcal F_C = \{ A \in \Sigma_T : \mu(C \setminus \psi^{-1}(A)) = 0 \}.
    \]
    We define the \term{family} of $C$, written $\family C$, as
    \[
        \family C = \{ \psi^{-1}(X) : X \in \essmin \mathcal F_C \}.
    \]
\end{defn}

It is clear that $\family C$ cannot be empty, as $\psi^{-1}(\Omega_T)$ must
contain almost all of $C$. To be rigorous, we must argue that $\mathcal F_C$ is
closed under countable intersections so that it has a well-defined essential
minimum. To see this, let $\mathcal F$ be any countable subset of $\mathcal
F_C$. Define $D = \bigcap \mathcal F$. Then $D \in \Sigma_T$ since it is a
sigma-algebra, and we have
\begin{align*}
    \mu\left( C \setminus \psi^{-1}(D) \right) 
    & = \mu\left( C \setminus \psi^{-1}\left(\,\bigcap \mathcal F\right) \right),\\
    & = \mu\left( C \setminus \bigcap_{F \in \mathcal F} \psi^{-1}(F) \right),\\
    & = \mu\left( \, \bigcup_{F \in \mathcal F} C \setminus F \right),\\
    & = 0,
\end{align*}
where the last step follows because each $F$ has the property that $C \setminus
F$ is a null set, and the union of countably many null sets is null. Hence $D
\in \mathcal F_C$.

Also note that for any $A,A' \in \family C$, it must be that $\mu(A \symdiff A')
= 0$. This is because $A = \psi^{-1}(B)$ and $A' = \psi^{-1}(B')$ for some $B,B'
\in \essmin \mathcal F_C$. As seen above, $\mu_T(B \symdiff B') = 0$.  Since
$\psi^{-1}(B \setminus B') = \psi^{-1}(B) \setminus \psi^{-1}(B')$, it must be
that $\psi^{-1}(B) \symdiff \psi^{-1}(B') = A \symdiff A'$ is a null set.

\begin{claim}
    \label{claim:completion_disconnected}
    Let $(\Omega, \Sigma, \mu, W)$ be a graphon. Suppose $C \in \Sigma$ does not
    separate twins, and $S \subset C$ such that $0 < \mu(S) < \mu(C)$. If $W <
    \lambda$ on $S \times (C \setminus S)$, then there exists a set $\bar S
    \subset C$ such that $\bar S$ does not separate twins,
    $\mu(S \setminus \bar S) = 0$, and
    $W < \lambda$ almost everywhere on $\bar S \times (C \setminus S)$.
\end{claim}

\begin{proof}
    Define
    \[
        \hat S = \{ x \in S : W(x,y) < \lambda \text{ for almost every $y \in C
        \setminus S$} \}.
    \]
    Since $W < \lambda$ almost everywhere on $S \times (C \setminus S)$, it must
    be that $\mu(\hat S) = \mu(S)$; This is an application of Fubini's theorem.
    Let $\bar S = \psi^{-1}(\psi(S))$. It follows that $\bar S \subset C$, and
    for every $x \in \bar S$, $W(x,y) < \lambda$ for almost every $y \in C
    \setminus S$.  Furthermore, $\bar S$ does not separate twins, and $\bar S$
    contains $\hat S$ -- which is $S$, less a null set -- so $\mu(S \setminus
    \bar S) = 0$.
\end{proof}

\begin{prop}
    \label{prop:family_of_cluster}
    Let $(\Omega, \Sigma, \mu, W)$ be a graphon and suppose $C$ is a cluster in
    $W$. Let $\bar C \in \family C$. Then $\mu(C \symdiff \bar C) = 0$.
\end{prop}

\begin{proof}
    Let $J_T = (\Omega_T, \Sigma_T, \mu_T)$ be the corresponding twin measure
    space.  Let $\psi : (\Omega, \Sigma, \mu) \to J_T$ be the map taking $x \in
    \Omega$ to its class of twins. Let $\lambda$ be a level at which $C$ is a
    cluster.

    We know that $C \setminus \bar C$ is a null set, so we need only show that
    $\bar C \setminus C$ is null.  Suppose otherwise. That is, let $R = \bar C
    \setminus C$ and suppose $\mu(R) > 0$. This rules out the case that $\bar C$
    is an atom. Let $A$ be any subset of $R$ with positive measure.  There are
    two cases: (1) For some $\lambda' < \lambda$, $W < \lambda'$ almost
    everywhere on $A \times (\bar C \setminus A)$, or (2) for every $\lambda' <
    \lambda$, $W \geq \lambda'$ on some subset of $A \times (\bar C \setminus
    A)$ of positive measure.

    Suppose case (1) holds for some $\lambda'$. Then for almost all $a \in A$ it
    is true that $W(a,y) < \lambda'$ for almost every $y \in \bar C \setminus
    A$. That is, let 
    \[
        \hat A = \{ a \in A : W(a,y) < \lambda' \text{ for almost every } y
        \in \bar C \setminus A \}.
    \]
    Then $\mu(\hat A) = \mu(A)$ and $W < \lambda$ almost everywhere on $\hat A
    \times (\bar C \setminus \hat A)$. 
    Define $\bar A = \psi^{-1}(\psi(\hat A))$. There are two subcases: Either
    (1a) $\bar A \cap C$ is null, or (1b) it is of positive measure. 
    
    Consider the first subcase. Define $D = \psi(\bar C) \setminus \psi(\bar
    A)$. We will show that $\psi^{-1}(D)$ contains $C$ except for a set of zero
    measure, and so $\psi^{-1}(D) \in \family C$.  But as we will see,
    $\mu(\psi^{-1}(D)) < \mu(\bar C)$, which cannot be. We have
    \begin{align*}
        \psi^{-1}(D) &= \psi^{-1}(\psi(\bar C) \setminus \psi(\bar A))\\
                     &= \psi^{-1}(\psi(\bar C)) 
                        \setminus \psi^{-1}(\psi(\bar A))\\
                     &= \bar C \setminus \bar A
    \end{align*}
    where the last step follows since $\bar C$ and $\bar A$ do not separate
    twins. Therefore,
    \begin{align*}
        C \cap \psi^{-1}(D) 
        &= C \cap (\bar C \setminus \bar A)\\
        &= (C \cap \bar C) \cup (C \cap \bar A)
    \end{align*}
    But $C \cap \bar A$ is a null set, so $\mu(C \cap \psi^{-1}(D)) = \mu(C \cap
    \bar C) = \mu(C)$. This implies that $\mu(C \setminus \psi^{-1}(D)) = 0$,
    and hence $\psi^{-1}(D) \in \family C$. But $\mu_T(D) = \mu_T(\psi(\bar C)
    \setminus \psi(\bar A))$, and $\psi(\bar A) \subset \psi(\bar C)$ with
    $\mu_T(\psi(\bar A)) = \mu(\bar A) > 0$. Therefore, $\mu_T(D) <
    \mu_T(\psi(\bar C))$, and so $\mu(\psi^{-1}(D) < \mu(C)$. This cannot be,
    since all elements of $\family C$ differ only by null sets. Hence it
    cannot be that $\bar A \cap C$ is null.

    Suppose case (1b) holds, then. That is, suppose $\bar A \cap C$ is not null.
    Then for every $x \in \bar A \cap C$ it is true that $W(x,y) < \lambda'$ for
    almost all $y \in \bar C \setminus A$. In particular, since $C \setminus (A
    \cap C) \subset \bar C \setminus A$, we have that $W < \lambda'$ almost
    everywhere on $(\bar A \cap C) \times (C \setminus \bar A)$. This means that
    $C$ is disconnected at level $\lambda'$, which violates the assumption that
    $C$ is a cluster at $\lambda > \lambda'$.

    Both subcases lead to contradictions, and so (1) cannot hold. Therefore, it
    must be that case (2) holds: For every $\lambda' < \lambda$, $W \geq
    \lambda'$ on some subset of $A \times (\bar C \setminus A)$. Furthermore,
    this must hold for arbitrary $A \subset R$ with positive measure. This
    implies that $\bar C$ is connected at every level $\lambda' < \lambda$, and
    hence part of a cluster at level $\lambda$. To see this, let $S,T \subset
    \bar C$ such that $S$ has positive measure and $S \cup T = \bar C$. Without
    loss of generality, assume $A \cap S$ is not null -- if it is, swap $S$ and
    $T$. Then $T \cap (\bar C \setminus A)$ is not null.  Therefore $W \geq
    \lambda$ on some subset of $S \times T$ with positive measure -- namely, $(S
    \cap A) \times (T \cap (\bar C \setminus A))$. Since this holds for
    arbitrary $S$ and $T$, $\bar C$ is connected.

    Therefore, both cases lead to contradictions under the assumption that
    $\mu(R) > 0$. Hence $\mu(R) = 0$, and $\mu(C \symdiff \bar C) = 0$.
\end{proof}

\begin{prop}
    \label{prop:cluster_in_w_is_connected_in_twin_free}
    Let $(J,W)$ be a graphon, and suppose $(J_T, W_T)$ is a twin-free graphon
    such that $W = W_T^\psi$ almost everywhere, where $\psi$ maps $x \in J$ to
    its class of twins. Let $C$ be a cluster of $W$ at level $\lambda$. 
    Then $\psi(\family C)$ is connected in $W_T$ at every level $\lambda' <
    \lambda$.
\end{prop}

\begin{proof}
    Since $C$ is a cluster of $W$ and $W = W_T^\varphi$ almost everywhere, $C$
    is a cluster of $W_T^\varphi$. Suppose for a contradiction that there exists
    a $\lambda' < \lambda$ such that $\psi(\family C)$ is disconnected. There
    are two cases: $\psi(C)$ is an atom, or it is not.

    Suppose that $\psi(\family C)$ is a disconnected atom. This implies that
    $W_T < \lambda'$ almost everywhere on $\psi(\family C) \times \psi(\family
    C)$. But this means that $W_T^\psi < \lambda$ almost everywhere on
    $\psi^{-1}(\psi(\family C)) \times \psi^{-1}(\psi(\family C)) = \family C
    \times \family C$. But $\mu(C \symdiff \family C) = 0$, such that this
    implies $W_T^\psi < \lambda$ almost everywhere on $C \times C$. This
    contradicts the assumption that $C$ is a cluster, since it is disconnected
    at level $\lambda' < \lambda$.

    Suppose then that $\psi(\family C)$ is not an atom, but is disconnected.
    Then there exists a $J_T$-measurable set $S$ of positive measure such that
    $W < \lambda$ almost everywhere on $S \times (\psi(\family C) \setminus S)$.
    Then $W_T^\psi < \lambda$ almost everywhere on $\psi^{-1}(S) \times
    \psi^{-1}(\psi(\family C) \setminus S) = \psi^{-1}(S) \times (\family C
    \setminus \psi^{-1}(S))$. This implies that $\family C$, and hence $C$, is
    not a cluster at level $\lambda$, since it is disconnected at $\lambda' <
    \lambda$.

    Both cases lead to contradictions, and so it must be that $\psi(\family C)$
    is connected in $W_T$ at every level $\lambda' < \lambda$.
\end{proof}

\begin{claim}
    \label{claim:disconnected_non_separating}
    Let $(J,W)$ be a graphon and suppose that $C$ is a set of positive measure
    that does not separate twins. If $C$ is disconnected, then either $W <
    \lambda$ almost everywhere on $C \times C$, or there exists a set $\bar A$
    such that $W < \lambda$ almost everywhere on $\bar A \times (C \setminus
    \bar A)$, and $\bar A$ does not separate twins.
\end{claim}

\begin{proof}
    If $C$ is an atom then it must be that $W < \lambda$ almost everywhere on $C
    \times C$, by definition of disconnectedness. Hence assume that $C$ is not
    an atom. Then there exists a set $S \subset C$ of positive measure such that
    $W < \lambda$ almost everywhere on $C \setminus S$. It may be, however, that
    $S$ separates twins.

    Let $\bar S$ be as described in Claim~\ref{claim:completion_disconnected}
    such that $\bar S$ essentially contains $S$, $\bar S$ does not separate
    twins, and $W < \lambda$ almost everywhere on $\bar S \times (C \setminus
    S)$. There are two cases: $\mu(\bar S) < \mu(C)$, or $\mu(\bar S) =
    \mu(C)$. Suppose the first case holds. Then, since $\mu((C \setminus S)
    \setminus (C \setminus \bar S)) = 0$, we have that for every $x \in \bar S$, 
    $W(x,y) < \lambda$ for almost every $y \in C \setminus \bar S$. Therefore,
    $W < \lambda$ almost everywhere on $\bar S \times (C \setminus \bar S)$.
    This proves the claim for the first case, as $\bar A = \bar S$.

    Now suppose $\mu(\bar S) = C$, which is to say that $\bar S$ differs from
    $C$ by a null set. Since $W < \lambda$ almost everywhere on $\bar S \times
    (C \setminus S)$, it follows that $W < \lambda$ almost everywhere on $C
    \times (C \setminus S)$. By symmetry of $W$, we have $W < \lambda$ almost
    everywhere on $(C \setminus S) \times C$. This means that $W < \lambda$
    almost everywhere on $(C \times C) \setminus (S \times S)$. 
    
    Let $T = C \setminus S$. Then $W < \lambda$ almost everywhere on $T \times
    C = (C \setminus S) \times C$. Let $\bar T$ be the set described in
    Claim~\ref{claim:completion_disconnected}, such that $\bar T$ essentially
    contains $T$, $\bar T$ does not separate twins, and $W < \lambda$ almost
    everywhere on $\bar T \times C$.

    There are two subcases: First, it may be that $\mu(\bar T) = \mu(C)$. If so,
    then $W < \lambda$ almost everywhere on $C \times C$, and we are done.
    Second, it may be that $\mu(\bar T) < \mu(C)$. In this case, we have $W <
    \lambda$ almost everywhere on $\bar T \times (C \setminus \bar T)$, and so
    setting $\bar A = \bar T$ proves the claim.
\end{proof}

\begin{prop}
    \label{prop:cluster_in_twin_free_connected_in_w}
    Let $(J,W)$ be a graphon, and suppose $(J_T, W_T)$ is a twin-free graphon
    such that $W = W_T^\psi$ almost everywhere, where $\psi$ maps $x \in J$ to
    its class of twins. Let $C$ be a cluster of $W_T$ at level $\lambda$. Then
    $\psi^{-1}(C)$ is connected in $W_T^\psi$ (and hence also $W$) at every
    level $\lambda' < \lambda$.
\end{prop}

\begin{proof}
    Suppose for a contradiction that $\psi^{-1}(C)$ is disconnected in
    $W_T^\psi$ at level $\lambda' < \lambda$. There are two cases:
    $\psi^{-1}(C)$ is an atomic, or it is not.

    Suppose $\psi^{-1}(C)$ is an atom. Then $W_T^\psi < \lambda$ almost
    everywhere on $\psi^{-1}(C) \times \psi^{-1}(C)$. Then, since $\psi$ is
    measure preserving, this implies that $W_T < \lambda$ almost everywhere on
    $C \times C$, which violates the assumption that $C$ is a cluster. 

    So assume that $\psi^{-1}(C)$ is not an atom. Then by
    Claim~\ref{claim:disconnected_non_separating}, either $W_T^\psi < \lambda$
    almost everywhere on $\psi^{-1}(C) \times \psi^{-1}(C)$, or there exists a
    set $S \subset \psi^{-1}(C)$ such that $\mu(S) > 0$ and $W < \lambda$ almost
    everywhere on $S \times (\psi^{-1}(C) \setminus S)$, and, crucially, $S$
    does not separate twins.

    In the first case, $W < \lambda$ almost every on $\psi^{-1}(C) \times
    \psi^{-1}(C)$ implies that $W < \lambda$ almost everywhere on $C \times C$,
    which contradicts the fact that $C$ is a cluster at level $\lambda$ in
    $W_T$.

    Suppose, then, that $W < \lambda$ almost everywhere on $S \times
    (\psi^{-1}(C) \setminus S)$, where $S$ does not separate twins. Then $W_T <
    \lambda$ almost everywhere on $\psi(S) \times \psi(\psi^{-1}(C) \setminus
    S)$, and $\mu_T(\psi(S)) = \mu(S) < \mu_T(C)$, so that $C$ is disconnected
    at level $\lambda'$ in $W_T$. This contradicts the fact that $C$ is a
    cluster at level $\lambda$, and so this case cannot hold.

    It therefore must be that $\psi^{-1}(C)$ is connected in $W$ at every level
    $\lambda' < \lambda$.
\end{proof}

\begin{lemma}
    Let $(J,W)$ be a graphon, and suppose $(J_T,W_T)$ is its twin-free
    representation by the map $\psi$, such that $W = W_T^\psi$ almost
    everywhere. Let $C$ be a cluster of $W_T$ at level $\lambda$. Then
    $\psi^{-1}(C)$ is a cluster of $W$.
\end{lemma}

\begin{proof}
    We have seen in Proposition~\ref{prop:cluster_in_twin_free_connected_in_w}
    that $\psi^{-1}(C)$ is connected in $W$ at every level $\lambda' < \lambda$.
    This means that $\psi^{-1}(C)$ must be part of some cluster $D$ at level
    $\lambda$ in $W$. By Proposition~\ref{prop:family_of_cluster}, $\mu(D
    \symdiff \family D) = 0$ such that $\family D$ represents the same cluster
    as $D$, and by
    Proposition~\ref{prop:cluster_in_w_is_connected_in_twin_free}, $\psi(\family
    D)$ is connected at every level $\lambda' < \lambda$ in $W_T$. Since
    $\psi^{-1}(\psi(\family D)) = \family D$, and $\psi$ is measure preserving,
    we have $\mu_T(\psi(\family D)) = \mu(D)$. 
\end{proof}
